# Supplementary material for: CryptoNite: Revealing the Pitfalls of End-to-End Private Inference at Scale
Source: arXiv:2111.02583 source file (2022-07-18)
Supplement: Supplementary file 1 [file case1_tail_latency.tex]

\begin{figure*}
\centering
\subfloat[ResNet32]{\includegraphics[scale=0.25]{figures/r32_delphi_mean}}
\subfloat[VGG16]{\includegraphics[scale=0.25]{figures/vgg16_delphi_mean}} 
\subfloat[ResNet18]{\includegraphics[scale=0.25]{figures/r18_delphi_mean}}
\caption{Mean latency for ``Server-garbler'' protocol.}
\vspace{-1em}
\label{fig:Case1TailLatency}
\end{figure*}
