# Supplementary material for: CryptoNite: Revealing the Pitfalls of End-to-End Private Inference at Scale
Source: arXiv:2111.02583 source file (2022-07-18)
Supplement: Supplementary file 2 [file max_sustainable_throughput.tex]

% \begin{figure*}
% \centering
% \subfloat[ResNet-32]{\includegraphics[scale=0.28]{figures/r32_maximum_sustainable_throughput}} 
% \subfloat[VGG-16]{\includegraphics[scale=0.28]{figures/vgg16_maximum_sustainable_throughput}} 
% \subfloat[ResNet-18]{\includegraphics[scale=0.28]{figures/r18_maximum_sustainable_throughput}}
% \caption{Maximum sustainable throughput for ResNet-32, VGG-16, and ResNet-18 (a, b, and c respectively) evaluated on $32\times32$ image (CIFAR-100/10) over a simulation period of 24 hrs: Initially, at lower arrival rate, number of completed requests linearly increases with arrival rate; however, {\em saturates} beyond a certain arrival rate (called as maximum sustainable throughput) and none of the requests get served. We note that network with higher FLOPs saturates earlier and able to sustain relatively lower arrival rate than the networks with lower FLOPs. Here, the order of maximum sustainable throughput is ResNet-32 $>$ VGG-16 $>$ ResNet-18}
% \label{fig:MaxSustainableThroughput}
% \end{figure*}
