# Supplementary material for: CryptoNite: Revealing the Pitfalls of End-to-End Private Inference at Scale
Source: arXiv:2111.02583 source file (2022-07-18)
Supplement: Supplementary file 3 [file mean_latency_with_throughput.tex]

% \begin{figure*}
% \centering
% \subfloat[ResNet-32]{\includegraphics[scale=0.25]{figures/r32_mean_latency_throughput}}
% \subfloat[VGG-16]{\includegraphics[scale=0.25]{figures/vgg16_mean_latency_throughput}} 
% \subfloat[ResNet-18]{\includegraphics[scale=0.25]{figures/r18_mean_latency_throughput}}
% \caption{Mean (PI) latency as a function of arrival rate for ResNet-32, VGG-16, and ResNet-18 (a, b, and c respectively) evaluated on $32\times32$ image (CIFAR-100/10) over a simulation period of 24 hrs: Initially, at lower arrival rate, mean latency is constant and then increases {\em exponentially} and starts saturating (as none of the requests get served) beyond a certain higher arrival rate. We note networks with lower FLOPs are able to accommodate higher arrival rate with constant mean PI latency (here the order is ResNet-32 $>$ VGG-16 $>$ ResNet-18)}
% \vspace{-1em}
% \label{fig:Case2MeanLatency}
% \end{figure*}
